# Supplementary material for: First principles investigation of zb-TiSn: A promising narrow bandgap semiconductor
Source: arXiv:2505.18940 source file (2025-05-25)
Supplement: Supplementary file 1 [file supplementary_data_file.pdf]

# First principles investigation of zb-TiSn: A promising narrow bandgap semiconductor

Sudeep R[a], Sarojini M[a], and Uma Mahendra Kumar Koppolu[a,*]
[a]Department of Physics, School of Advanced Sciences,
Vellore Institute of Technology, Vellore 632014, Tamil Nadu, India

# 1 Ecut convergence for GPAW calculations

In the Figure 1, we are presenting the plane-wave expansion energy cutoff (ecut) convergence test for zb-TiSn. Accordingly, an ecut of 450 eV was adopted for all subsequent calculations. This test was performed using the GPAW code within the projector augmented-wave (PAW) framework.

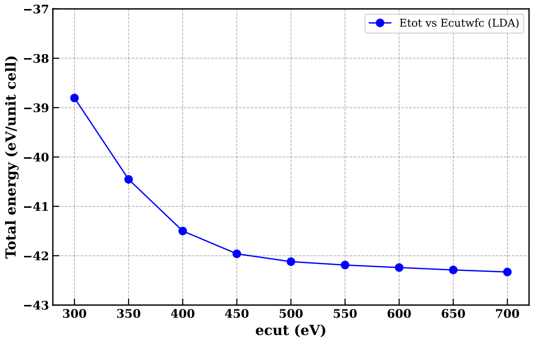


(a) LDA-PZ

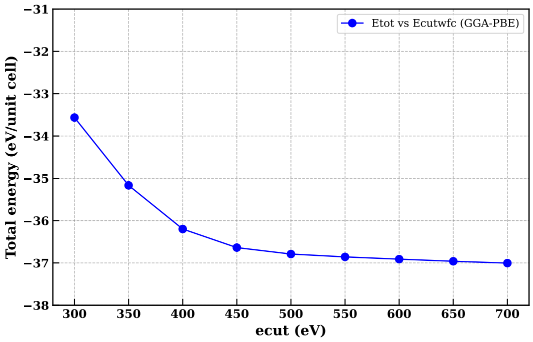


(b) GGA-PBE

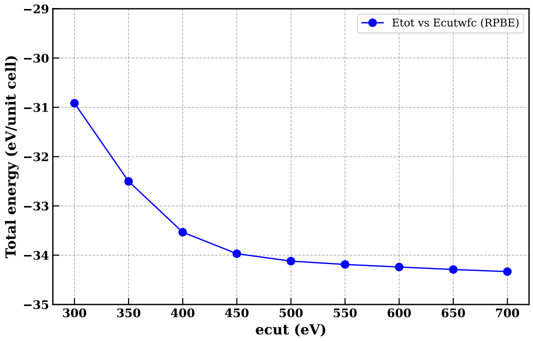


(c) GGA-RPBE

Figure 1: Ecut convergence using GPAW with a)LDA-PZ b)GGA-PBE c)GGA-RPBE.

# 2 Ecut convergence using QE

Quantum ESPRESSO calculations were carried out using two different exchange-correlation functionals. The Local Density Approximation (LDA-PZ) and the Generalized Gradient Approximation (GGA-PBE). The corresponding pseudopotentials, sourced from the PSLibrary version 1.0.0, are listed below.

- For LDA-PZ:
  - `Ti_pz_spn_rrkjus_psl.1.0.0.UPF`
  - `Sn_pz_dn_rrkjus_psl.1.0.0.UPF`
- For GGA-PBE:
  - `Ti_pbe_spn_rrkjus_psl.1.0.0.UPF`
  - `Sn_pbe_dn_rrkjus_psl.1.0.0.UPF`

The convergence test were performed by varying the cutoff energy and calculating the total energy. The test results are presented in Figure 2. From the Figure 2, it is evident that an energy cutoff of 60 Ry will be reasonable for all subsequent calculations with QE.

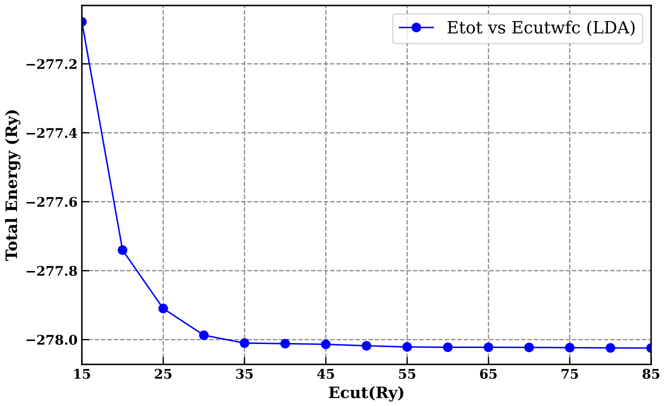


(a) LDA-PZ

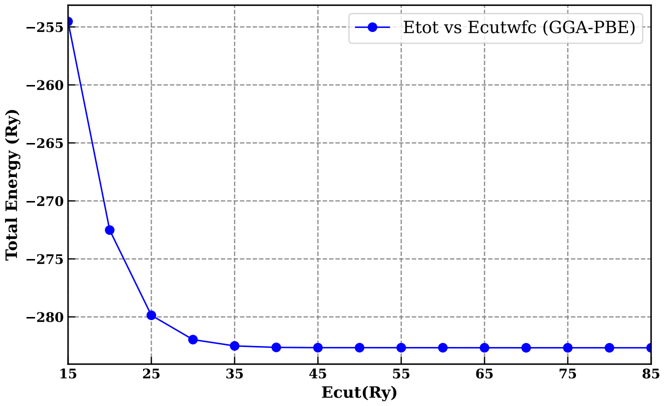


(b) GGA-PBE

Figure 2: Ecut convergence using QE with a)LDA-PZ b)GGA-PBE

# 3 k-point convergence using GPAW

In the Figure 3, we have presented the results of k-point convergence tests for zb-TiSn while using LDA-PZ, GGA-PBE, and GGA-RPBE exchange-correlation functionals. Based on this analysis, a $4 \times 4 \times 4$ $k$-point mesh was selected to ensure computational accuracy for all subsequent calculations.

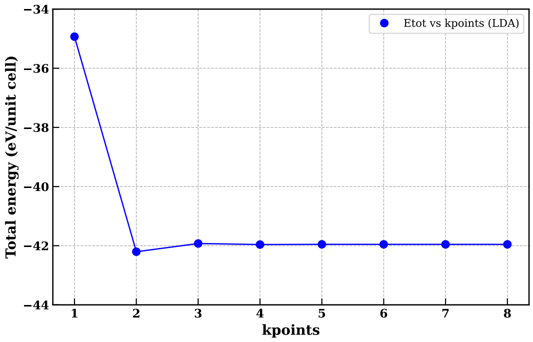


(a) LDA-PZ

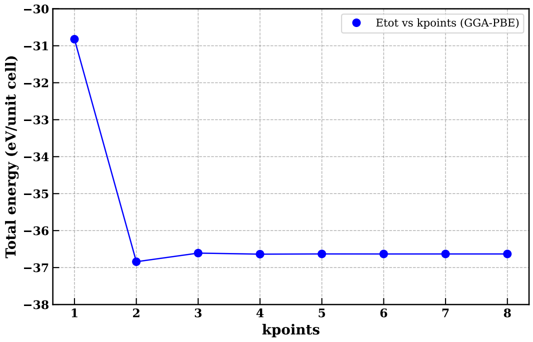


(b) GGA-PBE

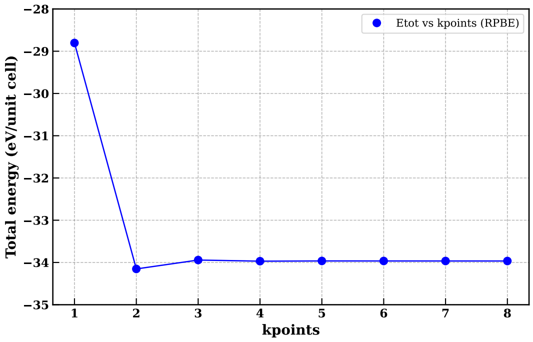


(c) GGA-RPBE

Figure 3: k-point convergence using GPAW with a)LDA-PZ b)GGA-PBE c)GGA-RPBE

## 4 k-points convergence using QE

In the Figure 4, Convergence of the total energy with respect to the $k$-point sampling was assessed by calculating the total energy using different $k$-point grids. For TiSn, an $8 \times 8 \times 8$ Monkhorst-Pack grid was employed to sample the Brillouin zone, ensuring sufficient accuracy and convergence of the electronic structure. These calculations were performed using both LDA-PZ and GGA-PBE exchange-correlation functionals.

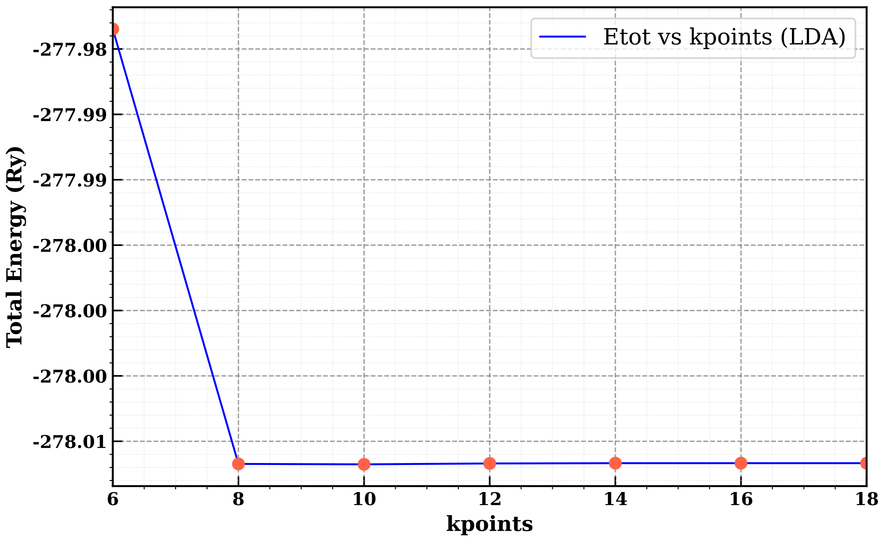


(a) LDA-PZ

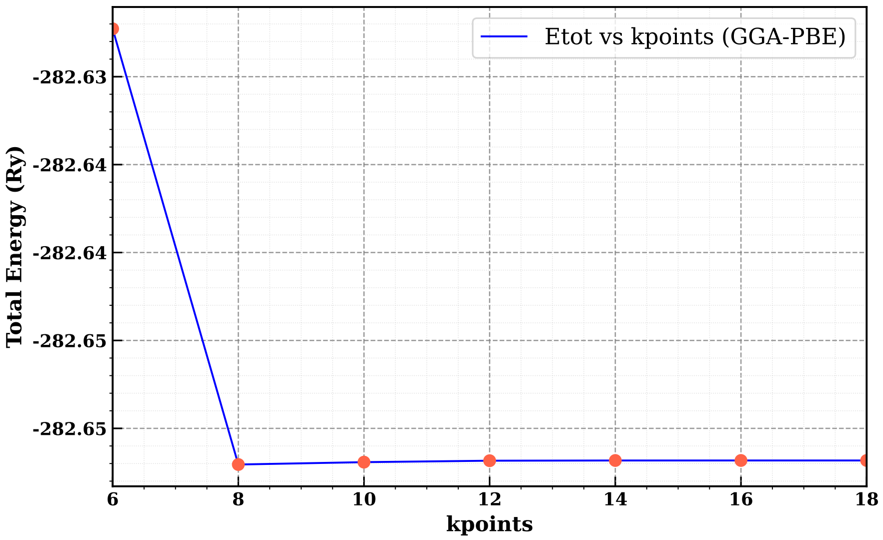


(b) GGA-PBE

Figure 4: k-point convergence using QE with a)LDA-PZ b)GGA-PBE

# 5 Hubbard-Correction GGA-PBE+U Calculations in GPAW

For the zb-TiSn system, applying a Hubbard 'U' correction to the Ti 3d orbitals, we have studied the effect of U on the lattice parameter and the band gap. The value of 'U' is varied from 2 eV to 6 eV. The equilibrium lattice constant was obtained by fitting total energy values to an energy–volume curve, ensuring that the structural parameters reflect the influence of on-site electron correlation at each level of 'U'. As well the variation in the band gap has been tabulated below in table 1.

| Hubbard U (eV) | a (Å) | Band gap (eV) |
|---|---|---|
| 2.0 | 6.34 | 0.30 |
| 3.0 | 6.37 | 0.30 |
| 4.0 | 6.39 | 0.31 |
| 5.0 | 6.40 | 0.32 |
| 6.0 | 6.41 | 0.33 |

Table 1: For the zb-TiSn, the applied Hubbard 'U' and corresponding lattice parameter and band gap are tabulated.

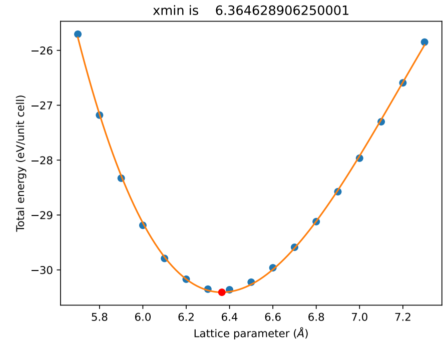


(a) U = 2 eV

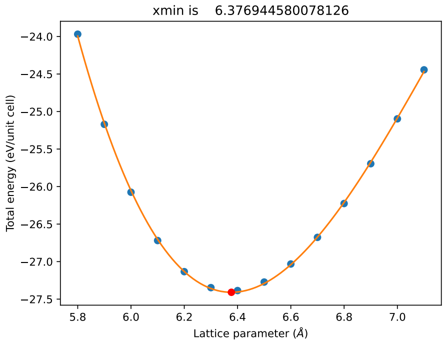


(b) U = 3 eV

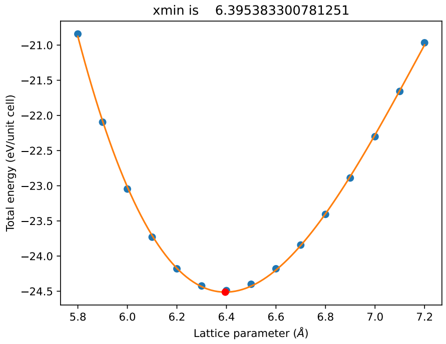


(c) U = 4 eV

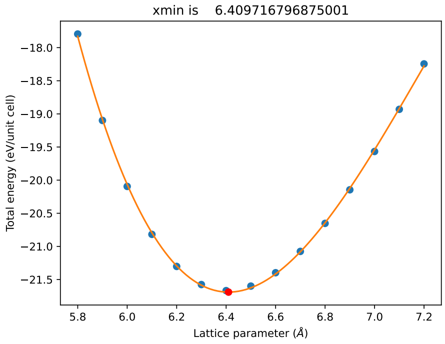


(d) U = 5 eV

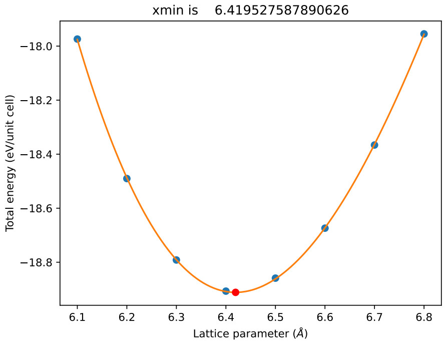


(e) U = 6 eV

Figure 5: Convergence of lattice constant for zb-TiSn using the GGA-PBE+U functional

# 6 Electronic band structure with GGA-PBE+U using GPAW

Using the optimized lattice constant and corresponding to each 'U' value, band structure calculations were subsequently performed to analyze the electronic properties of zb-TiSn. However, the results indicated that the band gap appeared to be very similar across the entire 'U' range, suggesting that the effect of Hubbard 'U' correction on the band gap energy is marginal in zb-TiSn.

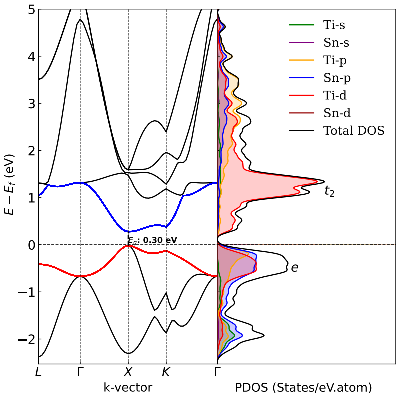


(a) U = 2 eV

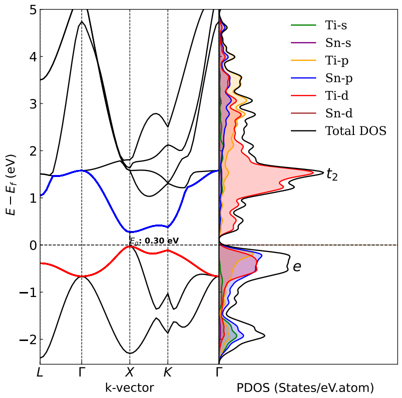


(b) U = 3 eV

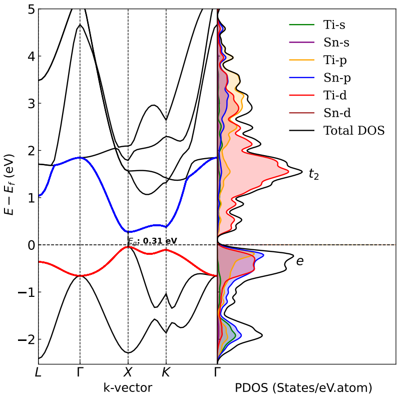


(c) U = 4 eV

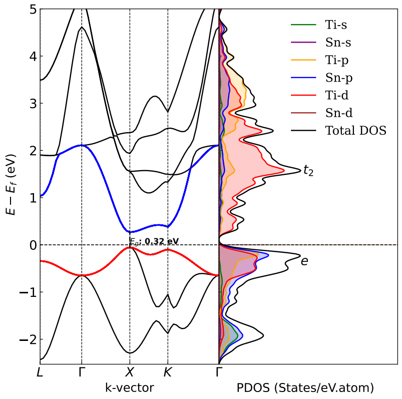


(d) U = 5 eV

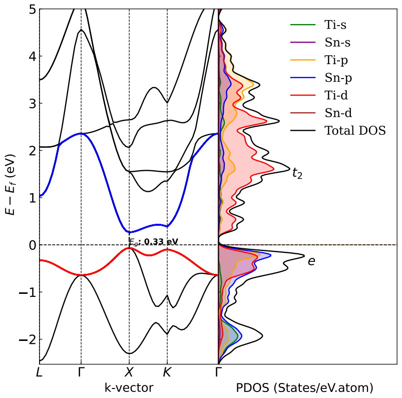


(e) U = 6 eV

Figure 6: Bandgap energy of zb-TiSn using the GGA-PBE+U functional.

# 7 GLLB-sc Functional

To assess the robustness of the electronic structure, calculations were performed using the GLLB-sc functional, which incorporates a derivative discontinuity correction which is absent in standard GGA-PBE and LDA-PZ functionals. The converged lattice constant

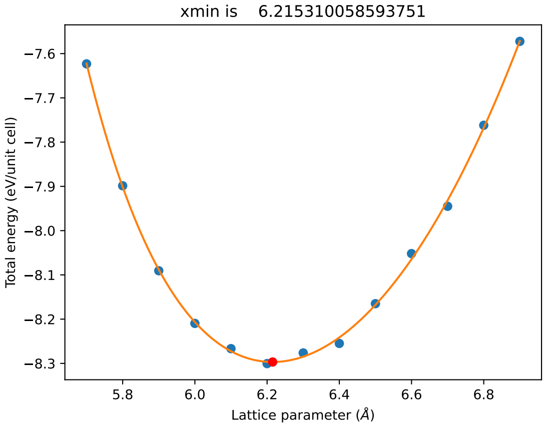


(a) Convergence testing of GLLB-sc functional

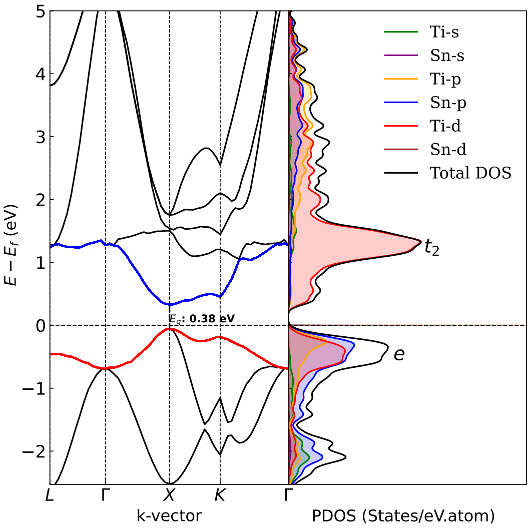


(b) Band Structure and PDOS of GLLB-sc functional

Figure 7: Using GLLB-sc functional a) lattice constant convergence b)electronic band structure and PDOS of zb-TiSn

was found to be 6.215 Å, and the calculated band gap was 0.38 eV. This band gap is in quantitative agreement with values obtained from LDA-PZ, GGA-PBE, and GGA-RPBE functionals, confirming the reliability of the results.

# 8 Optical Properties of GLLB-sc functional

Although the band gap calculated using the GLLB-sc functional differs only slightly ($\sim$ 0.06 eV) from those obtained with other functionals such as LDA-PZ, GGA-PBE, and GGA-RPBE, this minor variation does not lead to any significant changes in the linear optical response. The optical spectra, including absorption and dielectric functions, remain largely consistent across the different functionals. This suggests that the optical properties of zb-TiSn are relatively insensitive to minor variations in the band gap, further supporting the robustness of its electronic and optical behavior.

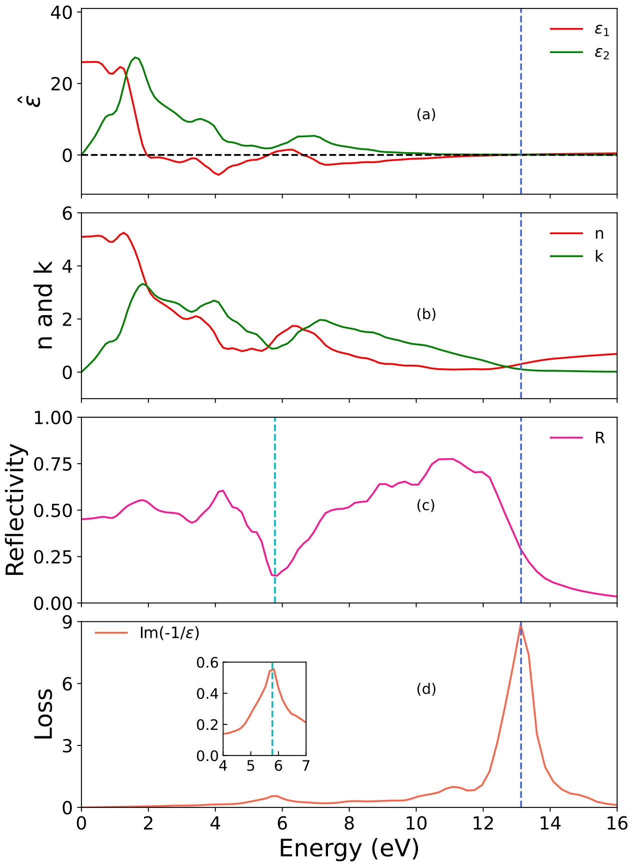

Figure 8: Optical properties of TiSn under GLLB-sc functional
(a) The real part $\varepsilon_1(\omega)$ and imaginary part $\varepsilon_2(\omega)$, (b) Refractive index $n$ and extinction coefficient $K$, (c) Reflectivity $R(\omega)$, and (d) Energy loss spectrum $L(\omega)$ are shown.

# 9 Absorption Spectrum

We have calculated the absorption spectrum of zb-TiSn using LDA, GGA-PBE, RPBE, and GLLB-sc functionals, all of which exhibit consistent absorption behavior across the wavelength range of 100 to 1500 nm. This consistency across different exchange–correlation functionals highlights the robustness and reliability of zb-TiSn's optical response. Such uniformity strengthens confidence in its potential for optoelectronic applications spanning the UV, visible, and NIR regions

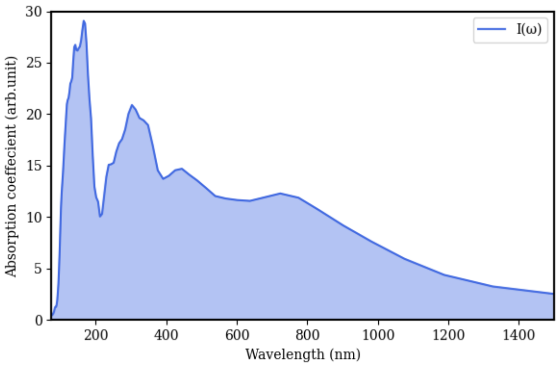


(a) LDA-PZ

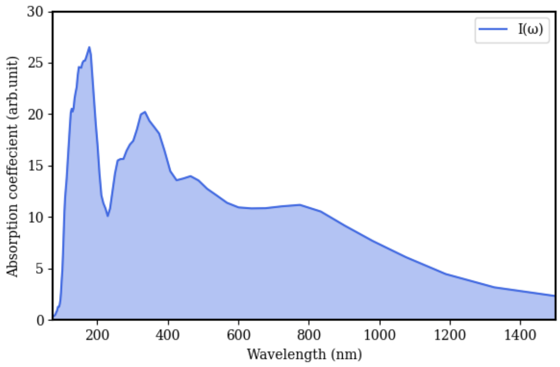


(b) GGA-PBE

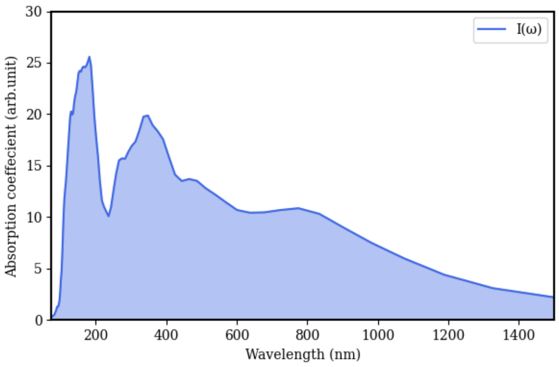


(c) GGA-RPBE

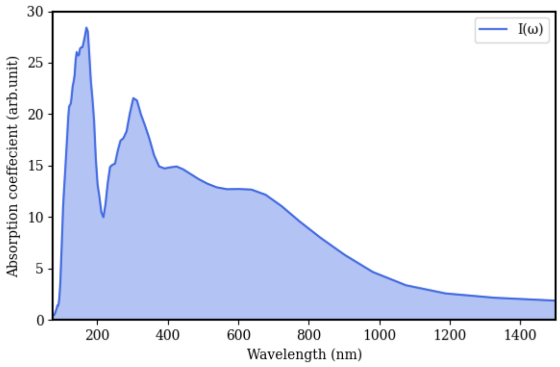


(d) GLLB-sc

Figure 9: Absorption spectrum of zb-TiSn for a)LDA-PZ b) GGA-PBE c)GGA-RPBE d)GLLB-sc
